# Supplementary material for: Prompt a Robot to Walk with Large Language Models
Source: arXiv:2309.09969 source file (2024-10-15)
Supplement: Supplementary file 1 [file appendix.tex]

\section*{APPENDIX}

\subsection{RL Training}

\subsection{Prompt example}
\label{apd:prompt}
